# Supplementary material for: Critical fragmentation properties of random drilling: How many random holes need to be drilled to collapse a wooden cube?
Source: arXiv:1601.03534 source file (2016-01-14)
Supplement: Supplementary file 1 [file drilling_SM.pdf]

# Supplemental Material: Critical fragmentation properties of random drilling: How many random holes need to be drilled to collapse a wooden cube?

K. J. Schrenk, M. R. Hilário, V. Sidoravicius, N. A. M. Araújo, H. J. Herrmann, M. Thielmann, and A. Teixeira

## I. LOCATING THE DRILLING TRANSITION

To determine the position of the drilling transition, we consider in Fig. S1 the finite-size behavior of five different estimators:

- $\chi_\infty$ refers to the maximum in the standard deviation of the largest cluster size. This is the position of the peaks in the curves in Fig. S6.
- $M_2'$ is the position of the peak of the second moment, excluding the contribution of the largest cluster, as plotted in Fig. S7.
- $\Pi_i(L)$ is the value of $p$ where the curves of $\Pi(L,p)$ and $\Pi(L/2,p)$, i.e. the spanning probabilities seen in Fig. S2, intersect [1].
- $\Pi$ is the average value of $p$ where the first cluster spanning the lattice in $z$-direction appears [2].
- $J$ is the point where the largest change in size of the largest cluster occurs, for every given sample, averaged over all samples [3].
- $K1$, $K2$, and $K3$ are the values obtained by Y. Kantor using Monte Carlo renormalization techniques [4].

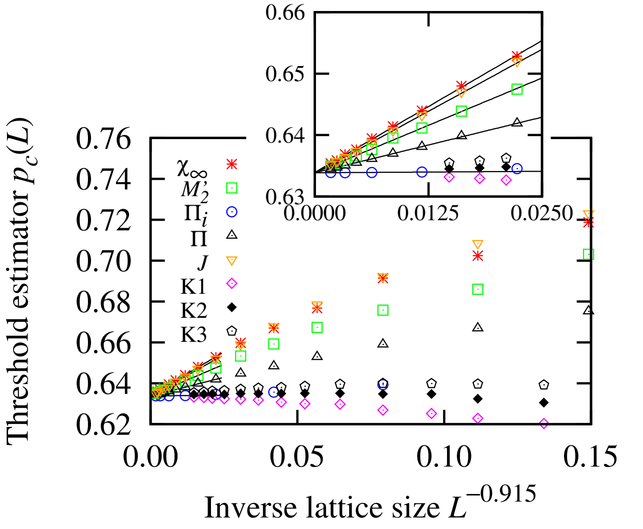


FIG. S1. Estimates for $p_c$ as a function of the inverse lattice size $L^{-0.915}$. Extrapolating to the thermodynamic limit yields $p_c = 0.6339 \pm 0.0005$. The data points are averages over at least 7700 samples (details in the text). Solid black lines are guides to the eye.

## II. DETAILED MODEL DESCRIPTION

Consider a simple cubic lattice of linear size $L$ with free boundary conditions. To explore different fractions of drilled holes, we use the following setup. In the initial configuration, there are no holes, such that all $N = L^3$ unit cells (sites) are present (occupied).

We consider the following process. On each face of the cube $i = x, y, z$ a site $\mathbf{x}_{0,i}$ is selected uniformly at random among the unselected sites, the corresponding hole is drilled, and all occupied sites in the direction perpendicular to the face and originating from $\mathbf{x}_{0,i}$ are removed (labeled as unoccupied). Therefore, in this step all occupied sites with coordinates $\mathbf{x}_{k,i} = \mathbf{x}_{0,i} + k\mathbf{e}_i$ are removed, where $\mathbf{e}_i$ is the unit vector perpendicular to the cube face and $k = 0, \ldots, L-1$, such that at most $L$ sites can be drilled in one step. This step is executed $3L^2$ times until all holes have been drilled and consequently all sites in the system are gone. If we denote by $(1 - p_i)$ the fraction of drilled holes in face $i$, we can characterize the state of the process with the control parameter $p = p_x = p_y = p_z$. A system is considered to be connected if there exists a path of occupied nearest neighbors connecting two opposing faces of the cube, say in $z$ direction. Let us denote by $\Pi(p)$ the probability that the system is connected. Then, in the thermodynamic limit, $\Pi(p)$ is a step function with $\Pi(1) = 1$ and $\Pi(0) = 0$ and with a transition at $p = p_c$ [15]. In Fig. S2 we see the connection probability as a function of the control parameter $p$ for different linear system sizes $L$. It can be observed that the curves intersect around $p_c = 0.6339 \pm 0.0005$ (see also Fig. S1). Given its error bars, this value of $p$ is higher than the site percolation threshold for the square lattice $p_c = 0.59274621 \pm 00000013$ [1, 16, 17] and lower than the cubic root of the site percolation threshold of the simple-cubic lattice: $[p_c(\text{s.c.})]^{1/3} \approx 0.67795$ [6].

## III. OBSERVABLES AS FUNCTION OF $p$

The connection probability $\Pi(p)$ is measured as the ratio of samples that are connected at parameter value $p$ and the total number of samples. For example, if all holes have been drilled, we have $p = 0$ and $\Pi(0) = 0$, and likewise if no hole has been drilled, $\Pi(1) = 1$ (see Fig. S2).

TABLE I. Critical exponents. The first column shows the symbol of the exponent. The second column shows the results for the drilling transition). For comparison, literature values for two- and three-dimensional classical percolation are given in columns three and four [1, 5]. Here, $\beta/\nu$ is the exponent related to the order parameter, see Eq. (S1). $\gamma/\nu$ is the exponent related to the second moment [see Eq. (S7)] of the cluster size distribution and to the susceptibility [see Eq. (S3)]. $1/\nu$ is the inverse of the correlation length critical exponent, as determined from the finite size scaling of threshold estimators (see Fig. S1) [1, 6]. $\beta$ is the order parameter critical exponent, determined from the behavior $P_\infty \sim (p-p_c)^\beta$ [see Fig. 2(a)] [1]. $\gamma$ is the susceptibility critical exponent, determined from the behavior $M_2' \sim |p-p_c|^{-\gamma}$ (see Fig. 2) [1, 6]. $d_{RS}$ is the fractal dimension of the red sites in the backbone of the largest cluster [6–9]. $d_{SP}$ is the fractal dimension of the shortest path in the largest cluster [10]. $d_{BB}$ is the fractal dimension of the backbone of the largest cluster [11–14]. $\tau$ is the exponent of the cluster size distribution (see Fig. S11).

| Exp. | Drilling | Classic 2D | Classic 3D |
|---|---|---|---|
| $\beta/\nu$ | $0.50 \pm 0.04$ | $5/48 \approx 0.1042$ | $0.4774 \pm 0.0001$ |
| $\gamma/\nu$ | $2.04 \pm 0.05$ | $43/24 \approx 1.7917$ | $2.0452 \pm 0.0002$ |
| $1/\nu$ | $0.915 \pm 0.010$ | $3/4 = 0.75$ | $1.1450 \pm 0.0007$ |
| $\beta$ | $0.52 \pm 0.04$ | $5/36 \approx 0.1389$ | $0.4169 \pm 0.0004$ |
| $\gamma$ | $2.3 \pm 0.1$ | $43/18 \approx 2.3889$ | $1.7862 \pm 0.0013$ |
| $d_{RS}$ | $0.92 \pm 0.05$ | $3/4 = 0.75$ | $1.1450 \pm 0.0007$ |
| $d_{SP}$ | $1.30 \pm 0.05$ | $1.13077 \pm 0.00002$ | $1.3756 \pm 0.0006$ |
| $d_{BB}$ | $2.14 \pm 0.08$ | $1.6432 \pm 0.0008$ | $1.875 \pm 0.003$ |
| $\tau$ | $2.1 \pm 0.1$ | $187/91 \approx 2.0549$ | $2.18925 \pm 0.00005$ |

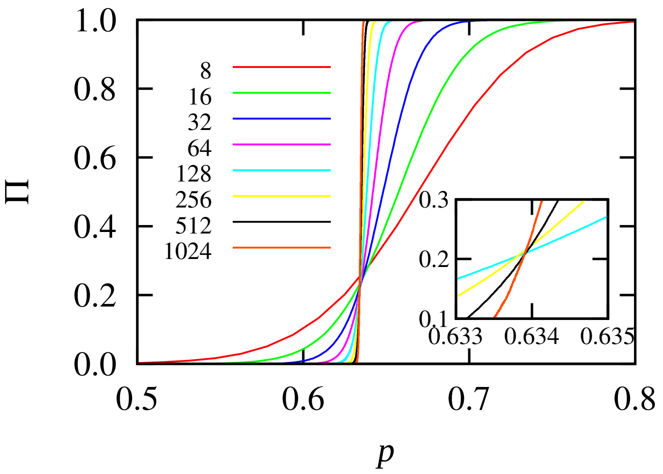


FIG. S2. Connection probability $\Pi$ as a function of the control parameter $p$. The systems consist of $N = L^3$ sites where the largest considered linear system size is $L = 1024$ and the smallest one is $L = 8$. Results have been averaged over at least $10^7$ samples for the smallest lattice size and $10^4$ samples for the largest one. $\Pi$ is measured as the fraction of connected samples. The curves for large lattices cross around $p_c = 0.6339 \pm 0.0005$ and $\Pi(p_c) = 0.21 \pm 0.03$. For clarity, the inset only shows the data for the four largest lattice sizes.

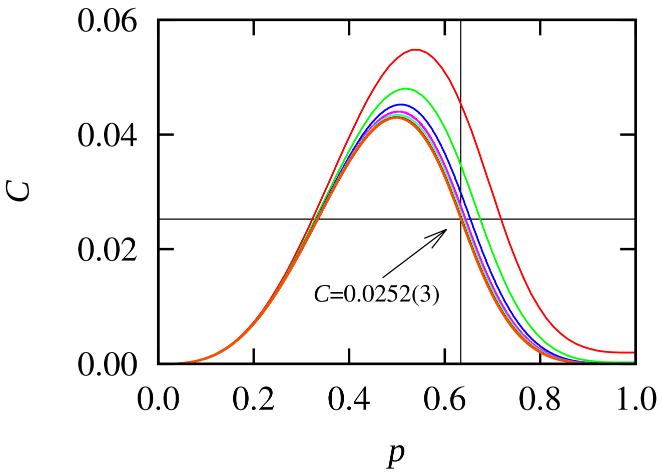


FIG. S3. Number of clusters per site $C$ as a function of the control parameter $p$. Lattice sizes and numbers of samples are the same as in Fig. S2. The curves seem to approach a limiting curve with increasing lattice size. The data extrapolates to $C(0.6339) = 0.0252 \pm 0.0002$ in the thermodynamic limit. The solid black straight lines are guides to the eye intersecting in $C(0.6339) = 0.0252$. The considered lattice sizes and colors of the curves are the same as in Fig. S2.

In the simple-cubic lattice, every site in the bulk has six nearest neighbor sites. If two occupied sites are nearest neighbors they are said to be connected. A set of connected occupied sites is called a cluster. Two distinct clusters are therefore separated by unoccupied sites. The number of sites forming the cluster is called its size. A single occupied site which has six unoccupied nearest neighbor sites is considered to be a cluster of unit size. The number of clusters per site $C$ is defined as the ratio of the number of distinct clusters and the total number of sites $N = L^3$. For critical percolation, this is known to be a lattice-dependent constant [21–24], the same seems to hold for the drilling transition, Fig. S3.

The largest cluster size per site $P_\infty$ is defined as the ratio of the maximum cluster size among all clusters in the system and the total number of sites $N = L^3$. For classical percolation, $P_\infty$ acts as order parameter [1] which is zero in the disordered state and nonzero in the ordered one. The data for the drilling transition is shown in Fig. S4. For percolation close to the percolation thresh-

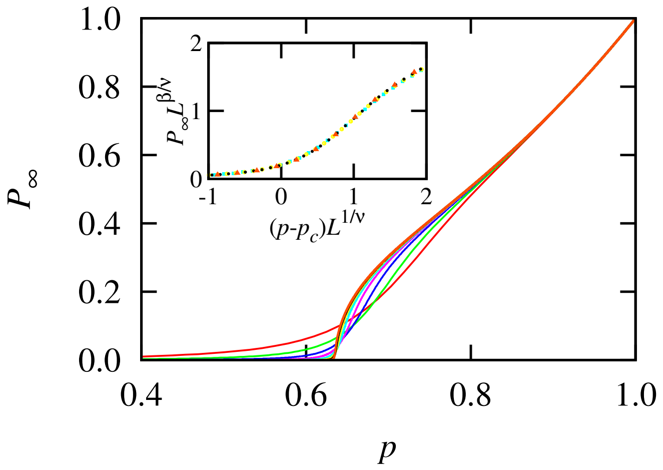


FIG. S4. Largest cluster size per site $P_\infty$ as a function of the control parameter $p$. In the insets, one sees the rescaled data for the four largest lattice sizes around $p_c$. We obtain a data collapse for $p_c = 0.6339$ and $1/\nu = 0.915$ and $\beta/\nu = 0.4774$, where $\beta/\nu$ is set to the value for three-dimensional percolation [6].

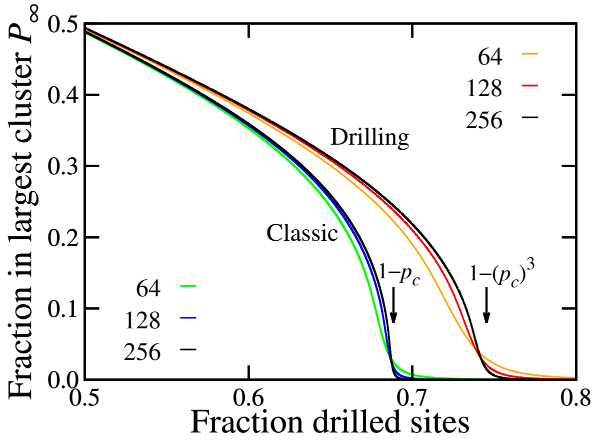


FIG. S5. Fraction of sites in the largest cluster $P_\infty$ as function of the fraction of sites that have been drilled, for drilling percolation (upper curves), and classical percolation (lower curves). For both models, data is shown for three different lattice sizes $L$. The arrows indicate $1 - p_c$, with $p_c$ the classical site percolation threshold, and $1-(p_c)^3$, respectively. For both models, this corresponds to the fraction of drilled sites at which the percolation transition occurs, in the thermodynamic limit. Results are averaged over $10^4$ samples.

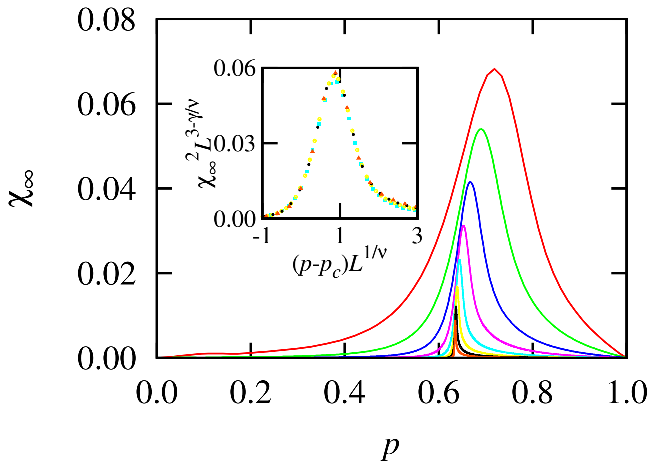


FIG. S6. Standard deviation of the largest cluster size per site $\chi_\infty$ as a function of the control parameter $p$. The inset shows the data for the four largest lattice sizes rescaled with $p_c = 0.6339$, $1/\nu = 0.915$, and $\gamma/\nu = 2.0452$. The ratio $\gamma/\nu$ is the one of three-dimensional percolation [6]. $1/\nu = 0.915 \pm 0.010$ is consistent with the scaling behavior of $P_\infty$ (see Fig. S4) and the estimators for $p_c$ (see Fig. S1), but it differs from the value for percolation, $1/\nu = 1.1450 \pm 0.0007$ [6, 18–20].

old, one expects the following scaling behavior:

$$P_\infty(p, L) = L^{-\beta/\nu} F_P[(p - p_c)L^{1/\nu}], \qquad \text{(S1)}$$

where $\beta$ is the critical exponent related to the order parameter, $\nu$ is the critical exponent related to the correlation length, $p_c$ is the percolation threshold, and $F_P$ is a scaling function [1]. If we compare classical percolation and drilling with respect to $P_\infty$ against the fraction of removed cells, we observe that the cube gets disconnected at lower fractions of removed cells in the case of classical percolation, see Fig. S5.

The standard deviation of the largest cluster size per site $\chi_\infty$ is defined as the square root of the variance of $P_\infty$:

$$\chi_\infty = \sqrt{\langle P_\infty^2 \rangle_S - \langle P_\infty \rangle_S^2}, \qquad \text{(S2)}$$

where $\langle \cdot \rangle_S$ indicates averaging over independent realizations (see Fig. S6). For percolation close to the percolation threshold, one expects the following scaling behavior:

$$\chi_\infty^2(p, L) = L^{-d+\gamma/\nu} F_\chi[(p - p_c)L^{1/\nu}], \qquad \text{(S3)}$$

where $d$ is the spatial dimension of the lattice, $\gamma$ is the critical exponent related to the susceptibility, and $F_\chi$ is a scaling function.

The second moment of the cluster size distribution is defined as

$$M_2 = \frac{1}{N} \sum_k s_k^2, \qquad \text{(S4)}$$

where the sum runs over all clusters in the system and $s_k$ is the size (number of sites) of cluster $k$. Excluding the contribution of the largest cluster size, we arrive at the following definition:

$$M_2' = M_2 - s_{\max}^2/N, \qquad \text{(S5)}$$

where $s_{\max}$ is the largest cluster size. In Fig. S7, we see

$$M_2'/N = M_2/N - s_{\max}^2/N^2. \qquad \text{(S6)}$$

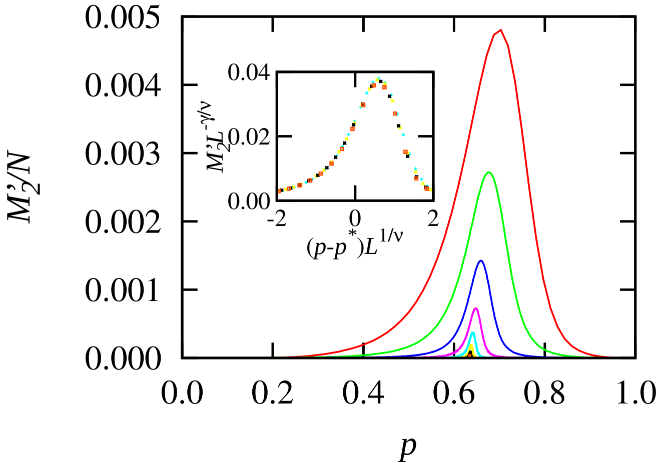


FIG. S7. Second moment of the cluster size distribution without the contribution of the largest cluster per site $M_2'/N$ as a function of the control parameter $p$. The inset shows the data for the largest four lattice sizes rescaled using the same values of $\gamma/\nu$, $1/\nu$, and $p_c$ as in Fig. S6.

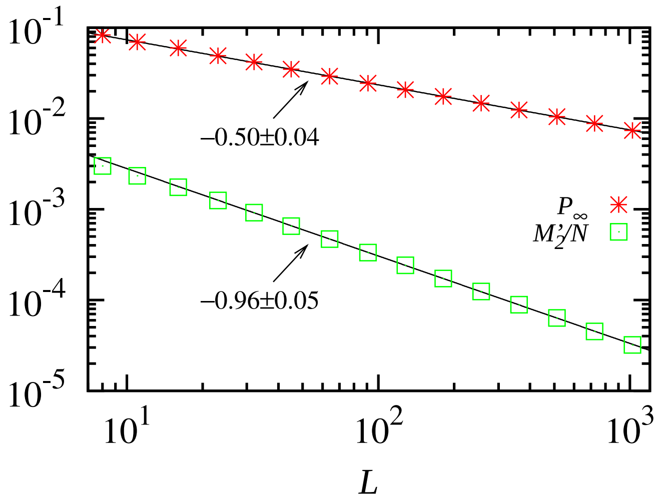


FIG. S8. Lattice size dependence of the largest cluster size per site $P_\infty$ and the second moment of the cluster size distribution without the contribution of the largest cluster per site $M_2'/N$ at $p = p_c = 0.6339$. The asymptotic slopes of the lines give $\beta/\nu = 0.50 \pm 0.04$ and $\gamma/\nu = 2.04 \pm 0.05$, in agreement with the reported values for three-dimensional percolation, $\beta/\nu = 0.4774 \pm 0.0001$ and $\gamma/\nu = 2.0452 \pm 0.0002$ [6].

Close to the percolation threshold, one expects the following scaling behavior:

$$M_2(p, L) = L^{\gamma/\nu} F_{M_2}[(p - p_c)L^{1/\nu}], \qquad \text{(S7)}$$

where $F_{M_2}$ is a scaling function. According to the scaling forms in Eq. (S1) and (S7), one expects to observe

$$P_\infty(p_c, L) \sim L^{-\beta/\nu} \qquad \text{(S8)}$$

and

$$M_2'(p_c, L)/N \sim L^{-d+\gamma/\nu} \qquad \text{(S9)}$$

at the threshold $p = p_c$. The corresponding measurements are shown in Fig. S8.

## IV. ALGORITHMS AND BOUNDARY CONDITIONS

To simulate the drilling model with an algorithm of complexity linear in the number of sites $N = L^3$, we adopt the following strategy. We consider initially a system with all sites occupied. Starting from this setup, the holes are drilled according to the processes described above. For each site, the fraction of drilled holes $(1 - p_x)$ at which it is removed is recorded. Once all holes have been drilled, we proceed in the opposite direction, and analyze the following percolation problem. Suppose we start from a lattice where all sites are unoccupied ($p_x = 0$). Now, $p_x$ is incremented and the sites of the lattice become occupied in the inverse order of the one in which they have been drilled. This procedure allows to keep track of the properties of the clusters of occupied sites as function of the control parameter $p_x$ [2, 16, 17]. Random numbers have been generated with the algorithms discussed in Refs. [29–31].

As a further test, we also considered alternative boundary conditions, obtaining results consistent with the ones obtained for free boundary conditions. In particular, we employed a single-cluster growth method, similar to the Leath algorithm for classical percolation [32, 33]. This method works at a fixed occupation probability $p$. We begin with a lattice of length $L$ equal to a small multiple of three. The holes in this initial cube are present with probability $1 - p$ and absent with probability $p$. If the site in the center of the lattice is occupied (this is the case with probability $p^3$), a cluster is grown starting from there, connecting to all occupied neighbors. In case the cluster touches a site on the boundary of the lattice, the linear lattice size is increased by a factor of three, the information on the drilled holes is accordingly propagated to the new lattice and the cluster growth continues. At a certain cutoff lattice size $L$, the cluster growth is terminated. This measurement gives the number of clusters as function of the size of the cluster at the origin, as shown in Fig. S10, at $p = p_c$. Because the probability of a randomly picked site to be in a cluster of size $s$ is proportional to $s$, this measures a size distribution which behaves as $sp(s)$. The corresponding power-law exponent is measured as $\tau - 1 = 1.165 \pm 0.01$, see Fig. S11. The influence of varying $p$ on the cluster size distribution is shown in Fig. S12. Finally we verified that the cutoff of the cluster size distribution, $s_{\mathrm{cut}}$, scales as expected from the fractal dimension of the largest cluster: We measured the fraction $f(L)$ of clusters grown from the origin that reach the boundary of a box of length $L$ and found that $f(L) \sim L^{-0.48\pm0.10}$ (not shown). One expects $f$ to be

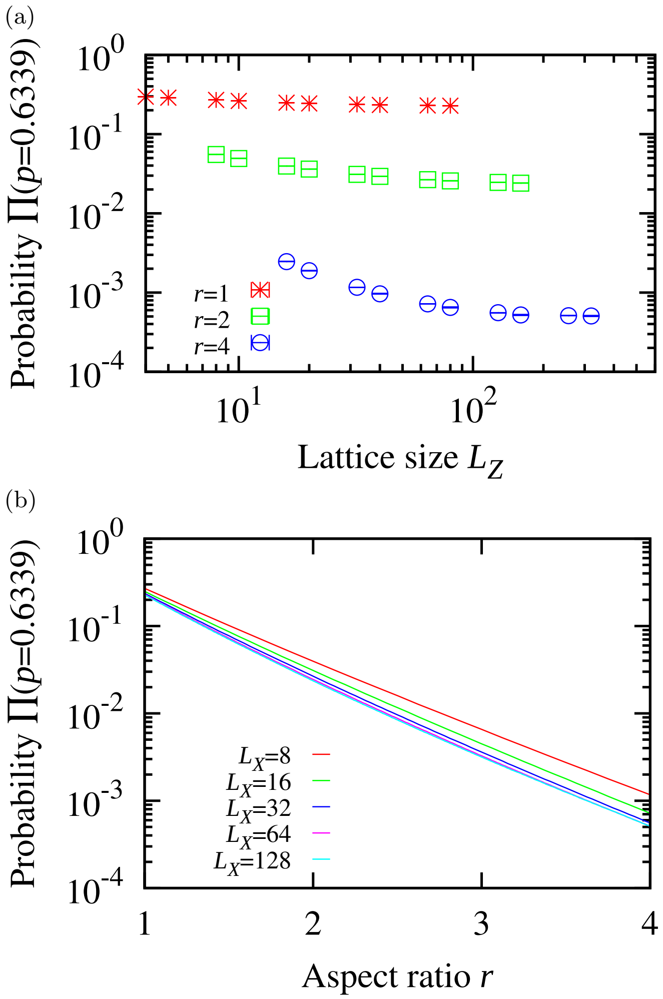


FIG. S9. (a) shows the connection probability $\Pi$ as function of the lattice length $L_Z$, with $p = 0.6339$, for different lattice aspect ratios $r$. $\Pi$ saturates to a constant for large $L_Z$. As can be seen in (b), for large aspect ratios $r$, the connection probability decays exponentially in $r$, similarly to classical percolation [25–28]. The lattice size is $L_X \times L_Y \times L_Z$ with $L_X = L_Y$ and $L_Z = rL_X$ and the connection probability is measured in $z$-direction. Results are based on at least $10^8$ samples.

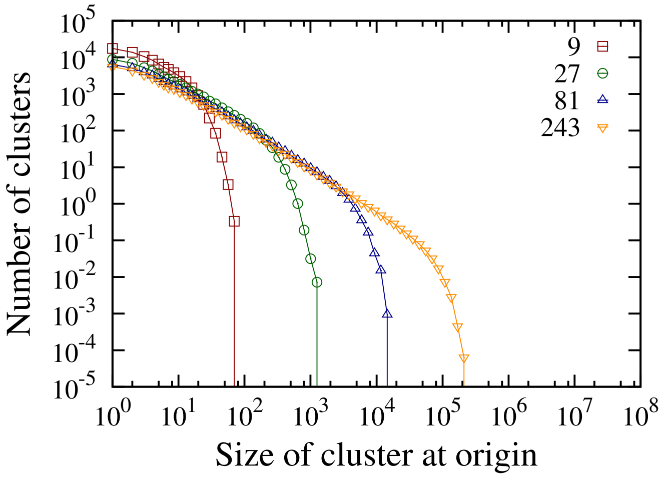


FIG. S10. Number of clusters of size $s$ versus size $s$ of the cluster at the origin, for $p = p_c$ and different values of the maximum considered lattice size. The histograms are obtained from $10^5$ clusters.

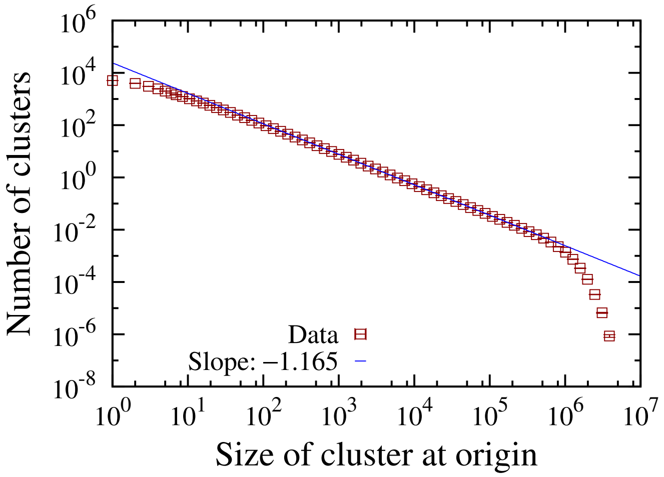


FIG. S11. Number of clusters of size $s$ versus size $s$ of the cluster at the origin, for $p = p_c$ and maximum lattice size 729. The data is obtained by averaging over $10^2$ histograms of $10^5$ clusters. The solid blue line is a guide to the eye with slope $-1.165$.

related to the cluster size distribution $p(s) \sim s^{-\tau}$ by

$$f(L) = \int_{s_{\mathrm{cut}}(L)}^{\infty} p(s) s \mathrm{d}s \sim L^{d_f - d}, \qquad \text{(S10)}$$

assuming $s_{\mathrm{cut}} \sim L^{d_f}$ [34, 35] and the validity of the scaling relation $\tau = 1 + d/d_f$ [1, 36], in analogy to classical percolation. In Fig. S8, we measure $d_f - d = -0.50 \pm 0.04$, in agreement with the behavior of $f$.

## V. CLUSTER SHAPE AND POWER-LAW DECAY

To study the geometry of the drilling transition clusters, we considered the eigenvalues and eigenvectors of the cluster inertia tensors [37–39], see Fig. S13 to S15. The results show that the clusters of the drilling transition are more anisotropic and aligned with the cube edges as the ones of classical 3D percolation.

We now present the details involved in the proof of the polynomial decay for the spanning probability $\Pi(p)$ as a function of the lattice length $L_X$ (recall that $L_Y = L_X$ and $L_Z = rL_X$ with a fixed aspect ratio $r$). We fix a $p \in (p_{2D}, p_c)$. We consider the diagonal band contained in the

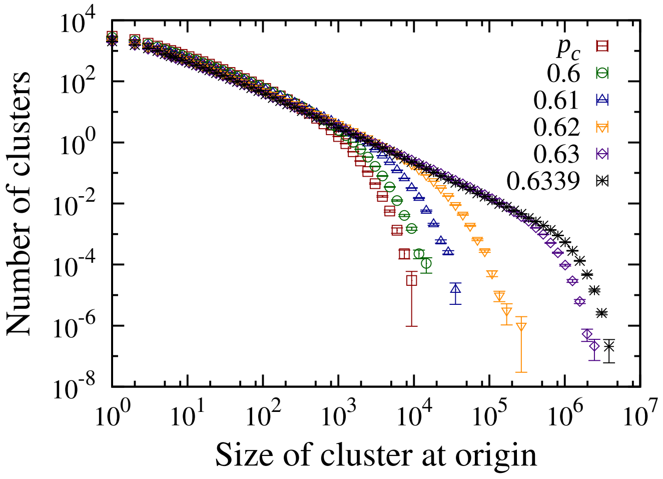


FIG. S12. Number of clusters of size $s$ versus size $s$ of the cluster at the origin, for different values of $p$. The data is obtained by averaging over 17 histograms of $4 \times 10^4$ clusters.

$(x, y)$-plane $B = \{(x, y);\ |x - L_X/2| \leq \alpha n \log(L_X/n), |x - y| \leq 2n\}$ and denote by $\tilde{B} = \{(x, y, z);\ (x, y) \in B, 0 \leq z \leq L_Z\}$. Recall the definition of the event $\mathcal{C}$ that there exists a path $\sigma$ contained in $\tilde{B}$ starting at height $z = 0$ and finishing at height $z = L_Z$ consisting of sites whose projections onto the $(x, y)$ and $(y, z)$-planes are free of holes. Our goal is to show that if $\alpha$ and $n$ are chosen sufficiently large then $\mathcal{C}$ has probability strictly larger than 0 uniformly in $L_X$, *i.e.* that there exists a $\delta > 0$ depending on $p$ and $r$ only, such that $P[\mathcal{C}] \geq \delta$. The argument involves a one-step renormalization. Let us consider the rectangles $B_X = [0, \alpha n \log(L_x/n)] \times [0, L_Z]$ and $B_Y = [0, \alpha n \log(L_Y/n)] \times [0, L_Z]$ contained in the $(x, z)$ and $(y, z)$-planes respectively. We tile $\tilde{B}$ with cubes of side length $n$, inducing a tiling of $B_X$ and $B_Y$ with squares of side length $n \ll L_X$. This allows us to see $B_X$ (respectively $B_Y$) as a rectangle in a renomalized square lattice whose sites correspond to $n \times n$ squares composed of $n^2$ sites of the original coordinate $(x, z)$ and $(y, z)$ planes respectively. For a given $n \times n$ square, we say that it is occupied if it is surrounded by a circuit of sites free of holes contained in its eight neighboring $n \times n$ squares (where two squares are considered neighbors if they intersect each other). Since $p > p_{2D}$ the probability that a square is occupied can be made arbitrarily high by choosing $n$ large enough. Thus we can choose $n$ and $\alpha$ large enough so that the probability of finding a path of cubes inside $B$ traversing it from bottom to top and whose projections are occupied squares in $B_X$ and $B_Y$ is strictly larger than 0 uniformly in $L_X$. Note that the fact that the projections are occupied squares, and the fact that the circuits of neighboring occupied squares intersect each other, assures that one can find a path inside $B$ like in the definition of the event $\mathcal{C}$.

(a)

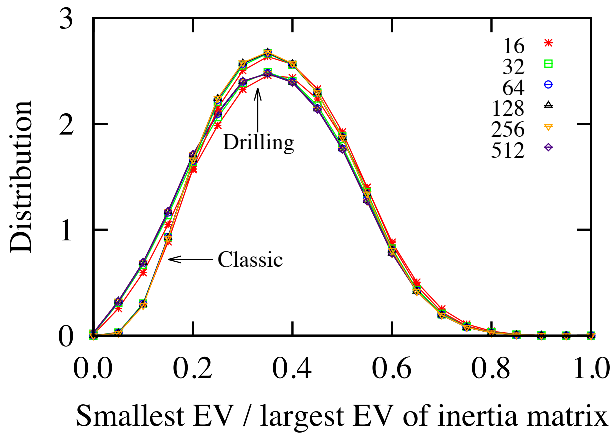


(b)

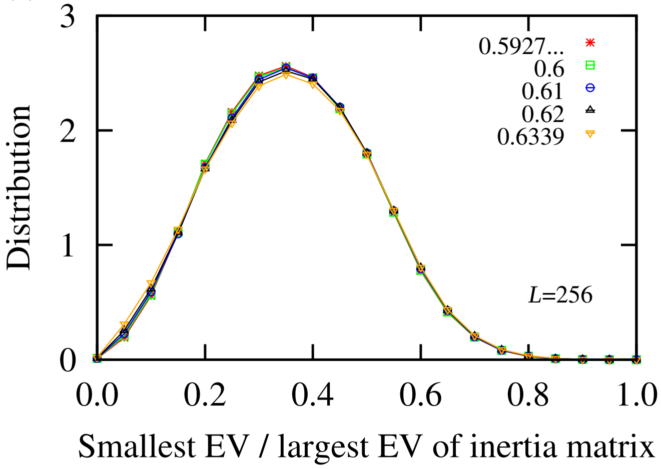


FIG. S13. (a) Histogram of the ratio of the smallest over the largest eigenvalue of the inertia matrix [40] for the drilling model ($p = p_c = 0.6339$) and classical percolation ($p = p_c = 0.3116077$ [6]) clusters in their center of mass frame, measured for different lattice sizes $L$, for all clusters with size at least 10. The inertia matrix consists of the following elements: $I_{ik} = \sum(x_l^2 \delta_{ik} - x_i x_k)$, where the sums are over all sites in the cluster. The different behavior of the left shoulders of the histograms indicates the relatively large amount of clusters with elongated shape in the drilling model. (b) Histograms as in (a), for the drilling model at different values of $p$ (and lattice size $L = 256$).

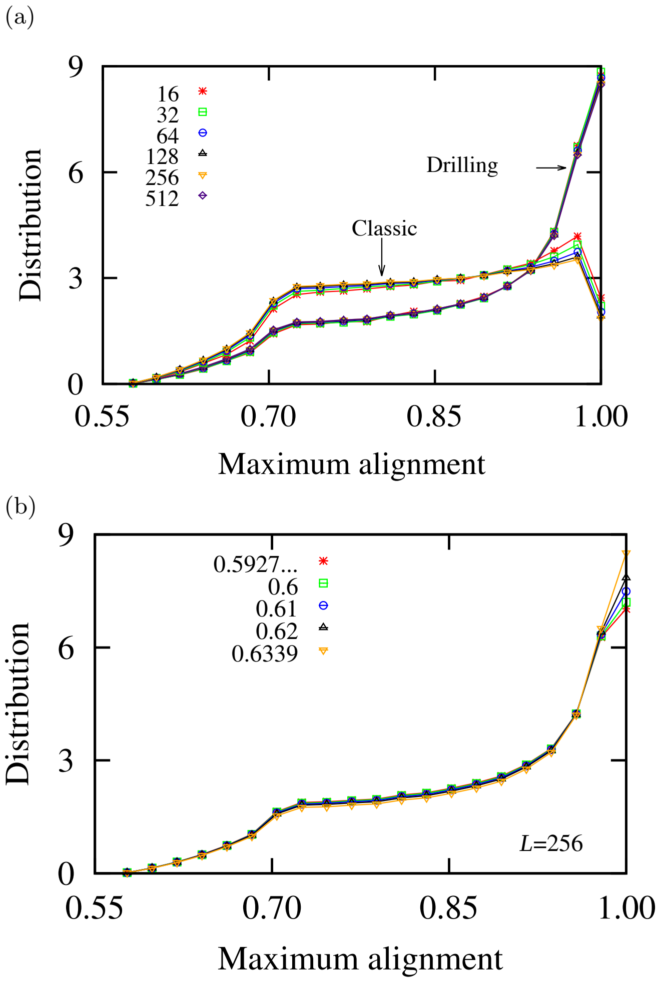


FIG. S14. (a) Histogram of the maximum alignment, with a coordinate axis, of the eigenvector of the inertia matrix with the smallest eigenvalue at criticality. We determine the eigenvector of the inertia matrix corresponding to the smallest eigenvalue. For each of the three coordinate axes, the absolute value of the cosine of the angle between the vector and the axis, $a_i$, is calculated. Then, the maximum alignment is defined as the highest $a_i$ for $i = x, y, z$. For the drilling model, the distribution of the maximum alignments shows a peak close to unity, corresponding to clusters whose anisotropy is aligned with the coordinate axes. (b) Histogram of alignments for the drilling model, for different values of the control parameter $p$ (and lattice size $L = 256$).

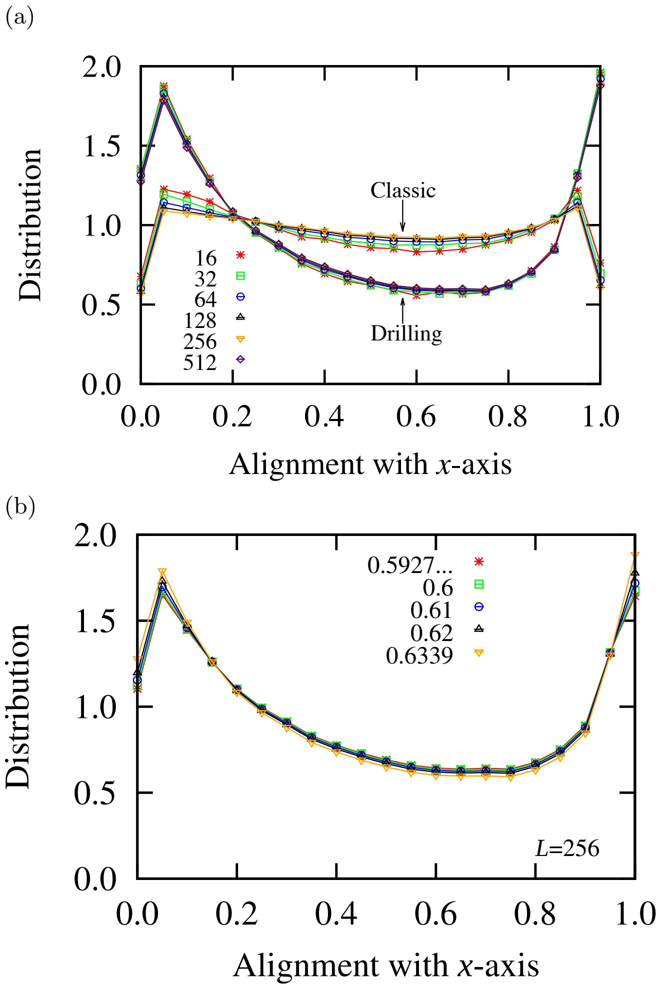


FIG. S15. (a) Similar data as in Fig. S14, however considering the alignment of the eigenvector with the lowest eigenvalue with a fixed coordinate axis (say, the $x$-axis, $a_x$). While the distribution of the alignment seems to become nearly uniform for classical percolation, for the drilling model one observes peaks close to zero and unity, compatible with the anisotropy of the clusters being aligned with the coordinate axes. (b) Alignment histograms as in (a), for the drilling model at different values of $p$ (and with lattice size $L = 256$).

[1] D. Stauffer and A. Aharony, *Introduction to Percolation Theory*, 2nd ed. (Taylor and Francis, London, 1994).
[2] R. M. Ziff, Phys. Rev. E **82**, 051105 (2010).
[3] J. Nagler, A. Levina, and M. Timme, Nat. Phys. **7**, 265 (2011).
[4] Y. Kantor, Phys. Rev. B **33**, 3522 (1986).
[5] S. Smirnov and W. Werner, Math. Res. Lett. **8**, 729 (2001).
[6] Y. Deng and H. W. J. Blöte, Phys. Rev. E **72**, 016126 (2005).
[7] A. Coniglio, Phys. Rev. Lett. **62**, 3054 (1989).
[8] O. Scholder, Int. J. Mod. Phys. C **20**, 267 (2009).
[9] K. J. Schrenk, N. A. M. Araújo, J. S. Andrade Jr., and H. J. Herrmann, Sci. Rep. **2**, 348 (2012).
[10] Z. Zhou, J. Yang, Y. Deng, and R. M. Ziff, Phys. Rev. E **86**, 061101 (2012).
[11] H. J. Herrmann and H. E. Stanley, Phys. Rev. Lett. **53**, 1121 (1984).
[12] P. Grassberger, Physica A **262**, 251 (1999).
[13] M. D. Rintoul and H. Nakanishi, J. Phys. A **27**, 5445 (1994).
[14] Y. Deng and H. W. J. Blöte, Phys. Rev. E **70**, 046106 (2004).
[15] M. Hilário, V. Sidoravicius, and A. Teixeira, arXiv:1202.1684.
[16] M. E. J. Newman and R. M. Ziff, Phys. Rev. Lett. **85**, 4104 (2000).
[17] M. E. J. Newman and R. M. Ziff, Phys. Rev. E **64**, 016706 (2001).
[18] C. D. Lorenz and R. M. Ziff, Phys. Rev. E **57**, 230 (1998).
[19] N. Jan and D. Stauffer, Int. J. Mod. Phys. C **9**, 341 (1998).
[20] H. G. Ballesteros, L. A. Fernández, V. Martín-Mayor, A. Muñoz Sudupe, G. Parisi, and J. J. Ruiz-Lorenzo, J. Phys. A **32**, 1 (1999).
[21] R. M. Ziff, S. R. Finch, and V. S. Adamchik, Phys. Rev. Lett. **79**, 3447 (1997).
[22] H. N. V. Temperley and E. H. Lieb, Proc. R. Soc. Lond. A **322**, 251 (1971).
[23] R. J. Baxter, H. N. V. Temperley, and S. E. Ashley, Proc. R. Soc. Lond. A **358**, 535 (1978).
[24] K. J. Schrenk, N. A. M. Araújo, and H. J. Herrmann, Phys. Rev. E **87**, 032123 (2013).
[25] J. L. Cardy, J. Phys. A **25**, L201 (1992).
[26] C. D. Lorenz and R. M. Ziff, J. Phys. A **31**, 8147 (1998).
[27] S. Smirnov, C. R. Acad. Sci. Paris I **333**, 239 (2001).
[28] S. Smirnov, in *Proceedings of the International Congress of Mathematicians, Madrid, Spain, 2006*, edited by M. Sanz-Solé, J. Soria, J. L. Varona, and J. Verdera (European Mathematical Society, Zürich, 2006) p. 1421.
[29] M. Matsumoto and T. Nishimura, ACM T. Model. Comput. S. **8**, 3 (1998).
[30] R. M. Ziff, Comput. Phys. **12**, 385 (1998).
[31] Boost C++ Libraries, `http://www.boost.org/`.
[32] P. L. Leath, Phys. Rev. B **14**, 5046 (1976).
[33] Z. Alexandrowicz, Phys. Lett. A **80**, 284 (1980).
[34] A. Margolina, H. J. Herrmann, and D. Stauffer, Phys. Lett. A **93**, 73 (1982).
[35] C. Borgs, J. T. Chayes, H. Kesten, and J. Spencer, Commun. Math. Phys. **224**, 153 (2001).
[36] H. Kesten, Commun. Math. Phys. **109**, 109 (1987).
[37] L. D. Landau and E. M. Lifschitz, *Mechanik*, fourteenth ed., Lehrbuch der Theoretischen Physik, Vol. 1 (Harri Deutsch, Frankfurt, 1997).
[38] J. Rudnick and G. Gaspari, Science **237**, 384 (1987).
[39] M. L. Mansfield and J. F. Douglas, J. Chem. Phys. **139**, 044901 (2013).
[40] Intel Math Kernel Library, `http://software.intel.com/en-us/intel-mkl`.
